# Supplementary material for: Nanosecond thermometry with Josephson junction
Source: arXiv:1704.04762 source file (2017-04-16)
Supplement: Supplementary file 1 [file Supplementary_Information_Nanosecond_thermometry.pdf]

# "Nanosecond thermometry with Josephson junction" Supplementary Information

M. Zgirski,[1*] M. Foltyn,[1] A. Savin,[2] M. Meschke[2] and J. Pekola[2]

[1]Institute of Physics, Polish Academy of Sciences,
Aleja Lotnikow 32/46, PL 02668 Warsaw, Poland,
[2]Low Temperature Laboratory, Department of Applied Physics,
Aalto University School of Science, P.O. Box 13500, 00076 Aalto, Finland

*To whom correspondence should be addressed; E-mail: zgirski@ifpan.edu.pl.

## Supplementary Note 1. Calibration curve $i_{sw}(T,\ P=0.5)$ extracted from S-curves measured at different bath temperatures

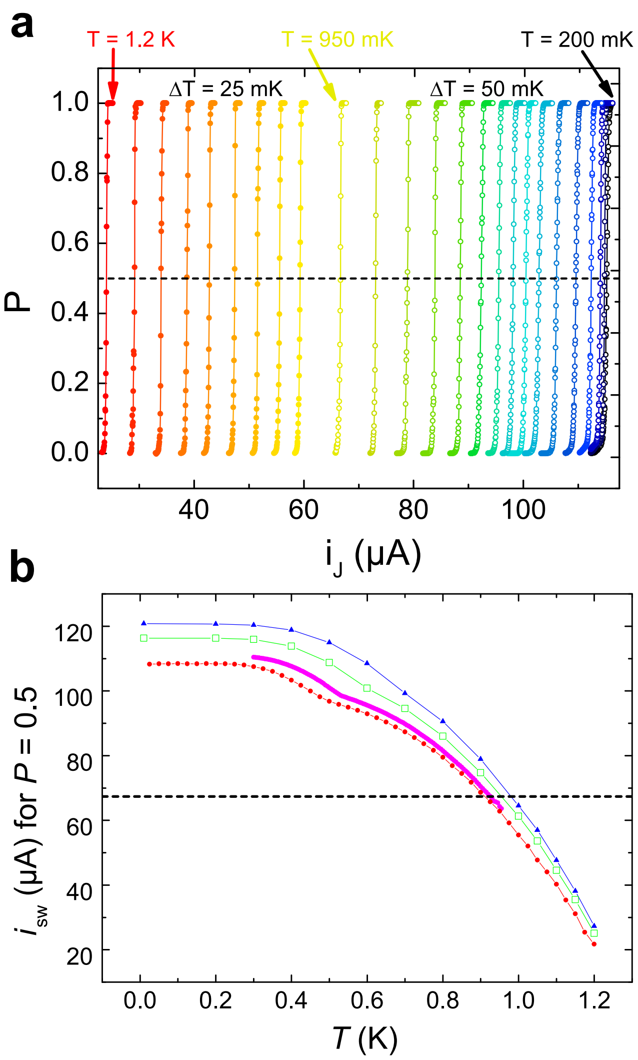


**Figure S1:** **(a)** A typical collection of S-curves measured at different temperatures used to extract switching current dependence on temperature (i.e. $i_{sw}(T)$ calibration curve). Points are experimental data and lines are guides for the eye. Dashed line corresponds to $P = 0.5$. **(b)** Temperature dependence of the switching current $i_{sw}(T)$ measured with different duration of the testing time $\tau_4$ of the pump&probe pulse (from top to bottom): 10ns, 50ns, 200ns, 1$\mu$s. The switching rate along each curve is: $6.9\cdot10^7$, $1.4\cdot10^7$, $3.5\cdot10^6$ and $6.9\cdot10^5$ Hz respectively. The dashed line is chosen to bring attention to temperature variation of the switching rate $\Gamma$ at a given current. This variation is important to understand switching dynamics in relaxation measurements when temperature during testing pulse is not constant (cf. Supp. Mat. Note 3).

## Supplementary Note 2. Relaxation of switching current - effect of pulse duration

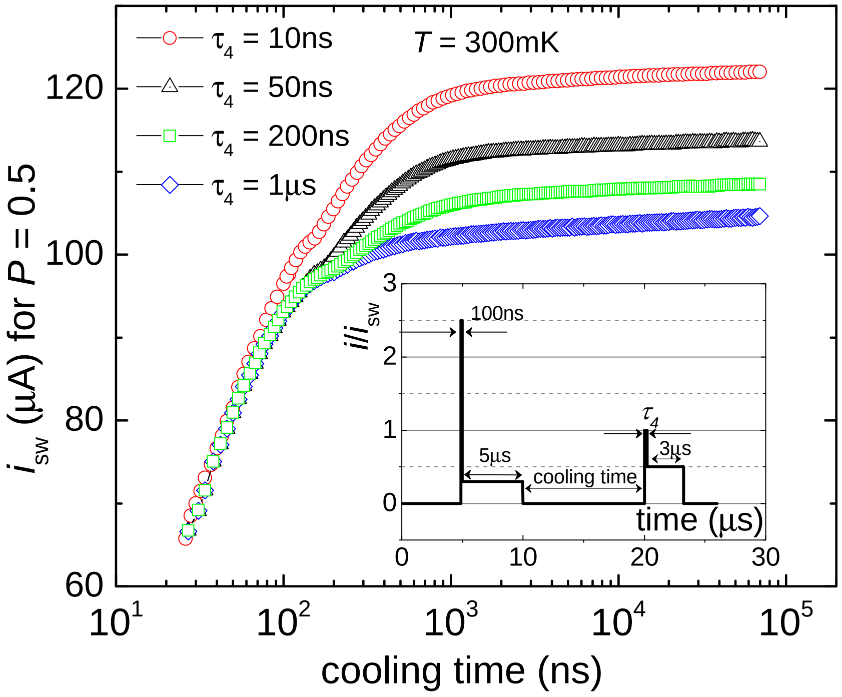


**Figure S2:** Relaxation of the switching current measured with different testing pulses. The testing part duration of the pump&probe pulse (time $\tau_4$) is (from top to bottom): 10ns, 50ns, 200ns, 1$\mu$s. Inset shows shape and timing for the pulse used in experiment.

The bridge can be tested with current pulses of different duration $\tau_4$. For measurements performed at constant temperature (with no relaxation) we expect to measure larger switching currents for shorter pulses. This directly follows from $P = 1 - exp(-\Gamma(i_b) \cdot \tau_4)$ relation (switching rate $\Gamma$ depends on the biasing current $i_b$). However, if switching is measured during fast thermal relaxation, we observe the same switching current independent of the duration of the testing pulse: for short enough cooling times relaxation curves $i_{sw}$ vs. cooling time are stuck on each other (Fig. S2). This is in fact a signature of very rapid decrease of temperature of the bridge. If in this case weak link does not switch to the normal state during first few nanoseconds its probability to switch at later times becomes exceedingly small owing to exponential dependence of the switching rate on temperature (Fig. S3.1a). As cooling rate is reduced the successive curves start to

depart from the rest with $\tau_4$=10ns curve separating first, $\tau_4$=50ns curve second etc.

## Supplementary Note 3. Conversion of the switching current into temperature

To convert switching current from relaxation curves into dynamic temperature we use calibration relationship $i_{sw}(T)$. However, doing so, some care is needed. To collect calibration curve we measured switching currents at constant temperatures whereas relaxation curves are acquired in a non-equilibrium condition: during the probing pulse the switching rate changes dramatically. The rate $\Gamma$ corresponding to the switching probability for the pulse of duration $\tau$, in equilibrium, verifies equation $P = 1 - exp(-\Gamma(T, i_b) \cdot \tau)$, where electron temperature $T$ and biasing current $i_b$ dependence of the rate has been displayed explicitly. The relation applied for different values of $\tau$ allows to extract an experimental rate dependence on the temperature for a fixed value of $i_b$. Such a dependence for the $i_b = 67.4\,\mu$A and the $P = 0.5$ is shown in the Figure S3.1a. When junction is tested while its temperature goes down the switching probability determination must involve integration over rates experienced by the junction during duration of the probing pulse $\tau_4$ i.e. in the time when junction temperature drops from $T_{start}$ to $T_{stop}$ (Fig. S3.1b):

$$P = 1 - exp\left(-\int_{0(T_{start})}^{\tau_4(T_{stop})} \Gamma(t, i_b)dt\right) = 1 - exp(-\Gamma_{av}(i_b) \cdot \tau)$$

$\Gamma_{av}(i_b)$ is the average switching rate during relaxation process equal to $\Gamma_0(T_0, i_b)$ achieved in the equilibrium for a known constant temperature, $T_0$, that can be readout from the $i_{sw}(T)$ calibration curve (we define $i_{sw} = i_b$ for $P = 0.5$). Since $\Gamma(T_{start}) > \Gamma_{av} = \Gamma_0(T_0) > \Gamma(T_{end})$ we conclude that $T_{start} > T_0 > T_{end}$ i.e. the junction reaches a well specified temperature $T_0$ in the time interval confined by the duration of the current pulse. We define the two limits for the time in which the actual temperature of $T_0$ is obtained: (i) $T_0$ is the temperature in the beginning of the current pulse, (ii) $T_0$ is the temperature in the end of the current pulse (Figure S3.2). Such an approach imposes the temporal uncertainty of the temperature determination equal to the pulse duration, but allows for a straightforward use of the calibration curve $i_{sw}(T)$ in recalculating of the

switching current into dynamic temperature. The AWG used in our experiment tailors the shortest pulses of about 10 ns duration but this number can be reduced by at least one order of magnitude with more advanced AWGs available in the market. We notice that it is possible to elaborate a more involved, switching model - dependent scheme for recalculating the switching current in terms of dynamic temperature, but the treatment above has the advantage of being straightforward and leaves no room for speculations.

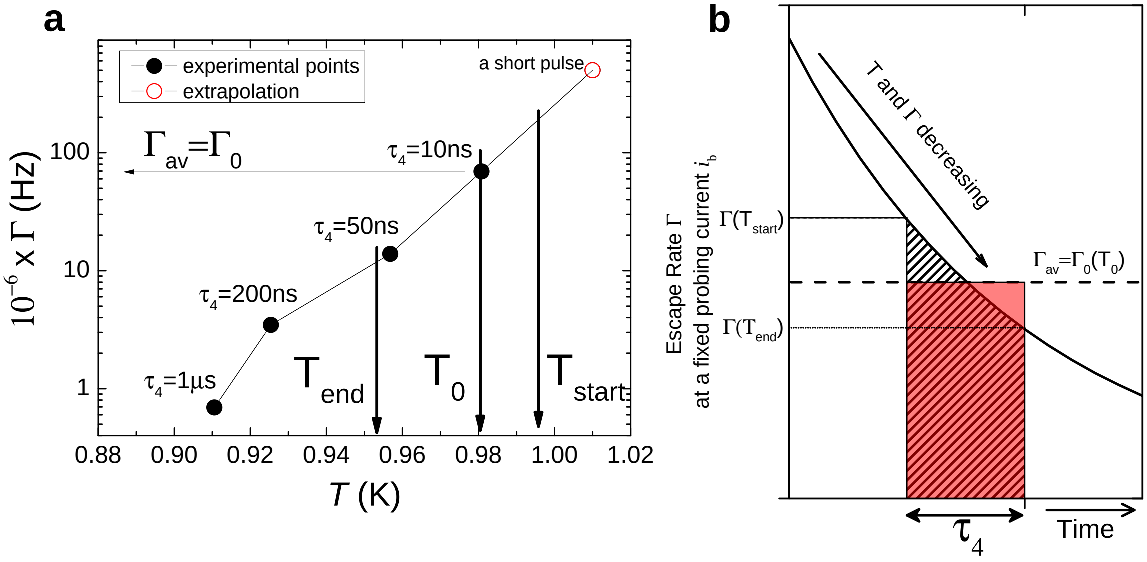


**Figure S3.1:** **(a)** Experimental temperature dependence of the switching rate at current of 67.4$\mu$A extracted with aid of the Fig. S1b. $T_{start}$ and $T_{end}$ denote temperatures of the bridge in the beginning and in the end of the $\tau_4$=10ns testing pulse, and were chosen here arbitrarily only for sake of demonstration. $T_0$ is an average temperature corresponding to an average rate $\Gamma_{av}$=$\Gamma_0$ – the one if the bridge was measured at constant temperature $T_0$. **(b)** Pictorial presentation of the temporal changes in the switching rate during testing pulse of duration $\tau_4$. Shaded areas are graphical representations of integrals: $\int_0^{\tau_4} \Gamma(t, i_b)dt$ and $\Gamma_{av}(T_0)\tau_4$.

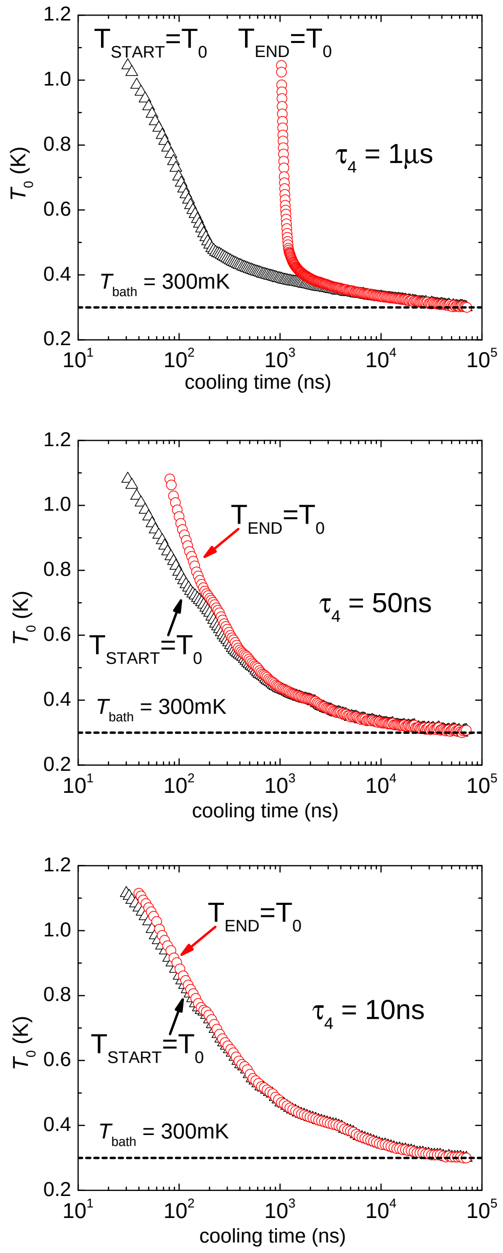


**Figure S3.2:** The effect of the testing pulse duration $\tau_4$ on the temporal resolution of determined temperature. We consider the two limits: the average temperature $T_0$ is lower limit estimation of temperature at the beginning of the testing pulse (black triangle curves) or upper limit estimation in the end of the testing pulse (red circle curves). It follows that $T_0$ must be reached in time confined by the two curves. For each pair curves are shifted by $\tau_4$. Resolution is limited by the "size of the probing tip".

## Supplementary Note 4. The graphical conversion of measured relaxation profile $i_{sw}$ vs. cooling time to temperature relaxation profile $T$ vs. cooling time with application of the calibration curve $i_{sw}(T)$

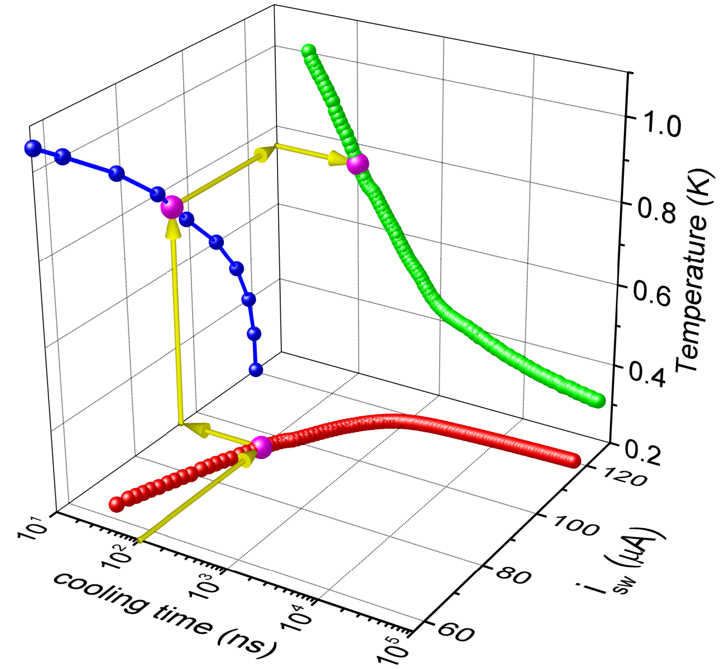


**Figure S4:** Transformation of the $i_{sw}$ vs. cooling time experimental profile into a temporal evolution of the temperature $T$ vs. cooling time with the application of a calibration curve $i_{sw}$(T). An exemplary conversion for a single point is displayed with arrows. The $i_{sw}$(T) curve bears information on values of the junction switching current at different electron temperatures. It is measured at fixed bath temperatures with electrons thermalized to the lattice.

## Supplementary Note 5. Retrapping mechanism in superconducting weak link

Figure S5 shows numerical temperature profiles for the superconducting wire biased with heating currents approaching a retrapping value. For higher biasing currents the calculated steady-state temperature profile is flat over entire wire except for its ends where it sharply descents towards the heat reservoir temperature. The calculation explains why after switching almost full length of the wire is above $T_c$ exhibiting a value of the resistance

very close to that measured at the bath temperature above $T_c$ (cf. I-V curves of the wire at 1.32 K and below $T_c$). Since the profile is flat in the center of the wire the dominant heat transfer under consideration is heat flow from hot electrons to phonons. It follows that the electron temperature of the central part of the wire (nanobridge) $T_e$ in a steady state with a constant current $i_b$ is the one for which Joule heating is balanced by the electron-phonon coupling: $\frac{r \cdot i_b^2}{S} = \sum(T_e^5 - T_{ph}^5)$. Owing to the strong power dependence the value of $T_e$ is not sensitive to overheating of phonons. The bridge enters superconducting state when amount of dissipated power at $T_e$=$T_c$ is smaller than the power transferred from electrons to phonons. It happens at $i_b = i_{ret} = \sqrt{S/r \cdot \sum(T_c^5 - T_{ph}^5)}$. In practice the retrapping current $i_{ret}$ is slightly larger, for the generated heat is conducted away also by the hot electron diffusion. Profiles were calculated with the Runge-Kutta method of $4^{th}$ order treating the two coupled $1^{st}$ order differential equations.

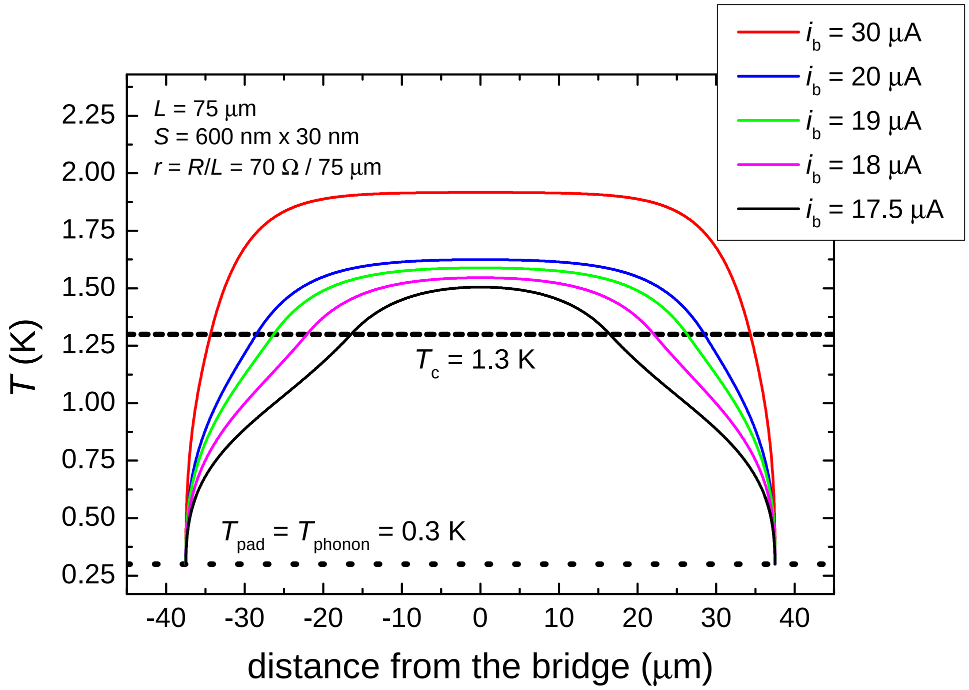


**Figure S5:** Steady state temperature profiles for superconducting nanowire biased with heating current of (from top to bottom): 30, 20, 19, 18 and 17.5 $\mu$A.

## Supplementary Note 6. Modeling temperature relaxation with ideal pads

We model heat relaxation assuming constant pad temperature equal to the bath temperature and compare the calculation with the experimental data (Fig. S6) We see that the model predicts faster temperature fall than the one measured in the experiment. We show also what would be the expected temperature decrease if one of the relaxation mechanisms did not exist. Green dashed curve was calculated assuming that heat relaxes only through hot electron diffusion, black dashed curve – only through electron-phonon coupling. We see that above 0.9 K electron-phonon relaxation channel dominates while below 0.6 K hot electron diffusion takes over as electron-phonon becomes very inefficient. The long relaxation tail in the experimental profile at $t > 1000$ns whose relaxation rate qualitatively resembles electron-phonon process, suggests that wire's pads, after switching, are heated above the bath temperature. Pads cool down predominantly due to electron-phonon coupling. We neglect the hot electron diffusion to find temperature evolution of the pads in a form convenient for the numerical integration.

$$-c_s(T_e) \cdot \frac{\delta T_e}{\delta t} = \dot{q}_{ep}(T_e)$$

$$t(T_e) = \int_{T_e}^{T_{e,0}} \frac{c_s(T^{'})}{\dot{q}_{ep}(T^{'})} dT^{'}$$

with $c_s(T_e)$ and $\dot{q}_{ep}(T_e)$ calculated numerically.

The modeling taking into account overheating of pads is displayed in the main text and, for higher starting temperature in Fig. S7.

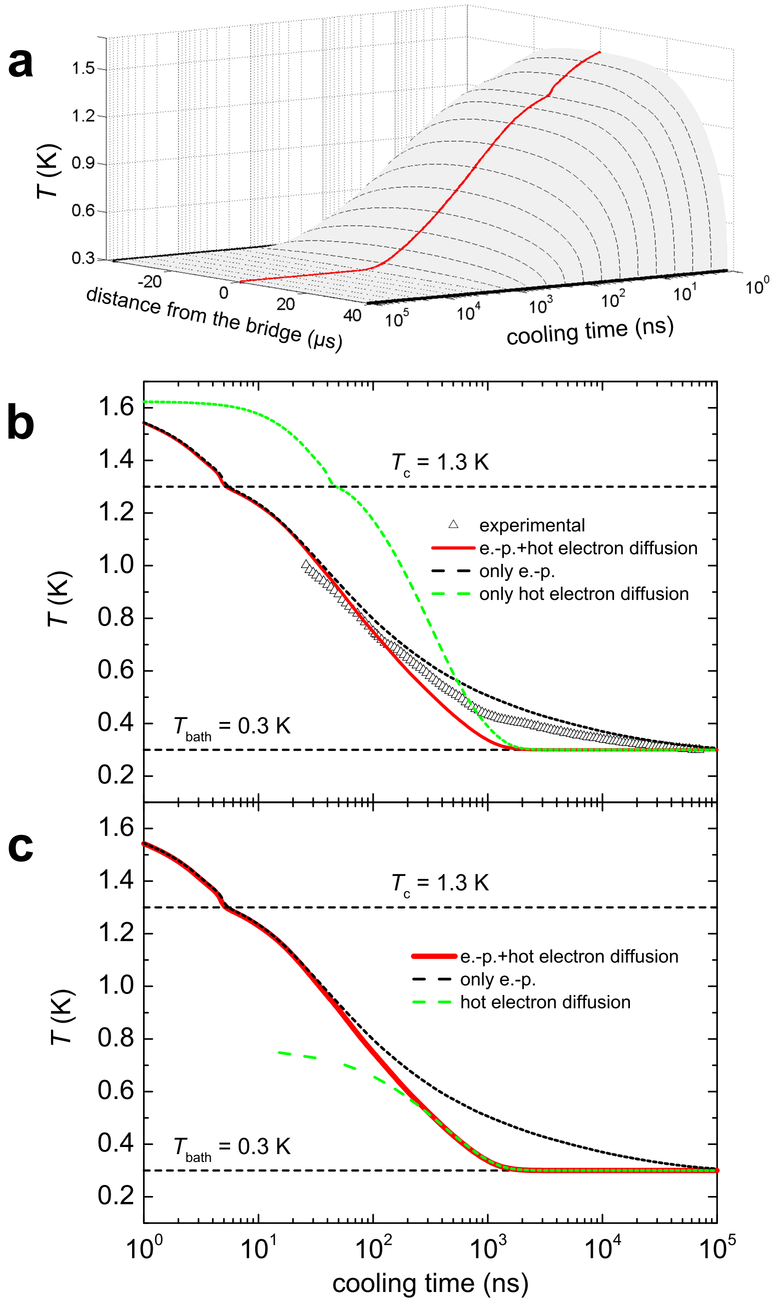


**Figure S6:** Numerical modeling of temperature relaxation in the superconducting nanowire connected to perfect energy reservoirs. **(a)** Temporal evolution of temperature profile in the wire. Temperature variations in the bridge are distinguished with red solid line. **(b)** Modeled bridge temperature for different relaxation mechanisms compared to experimental data. Cooling time=0 corresponds to the end of the heating pulse intended to bring the wire to a steady state with $T = 1.625\,\mathrm{K}$ in the center of the wire. Solid red line (the same as in panel (a)) shows evolution of the temperature if all mechanisms are accounted for. Two dashed curves show relaxation with only one channel of energy flow (electron-phonon or hot electron diffusion) **(c)** Two components of the simulated relaxation: electron-phonon coupling dominating above $0.9\,\mathrm{K}$ and hot electron diffusion dominating below $0.6\,\mathrm{K}$.

## Supplementary Note 7. Modeling temperature relaxation with overheated pads ($T_{start} = 3.3K$)

Amplitude of the current at the forced switching is about 116 $\mu$A elevating the temperature of the central part of the wire (nanobridge) to $T_e = 3.3\,\text{K}$; $\left(\dfrac{r \cdot i_b^2}{S} = \sum(T_e^5 - T_{ph}^5)\right)$. The fast relaxation within first microsecond involves processes leading to equalizing the temperature in the whole wire with the temperature of the pads. The slow relaxation reflects dynamics of the electron-phonon heat transfer in the pads (Figure S7).

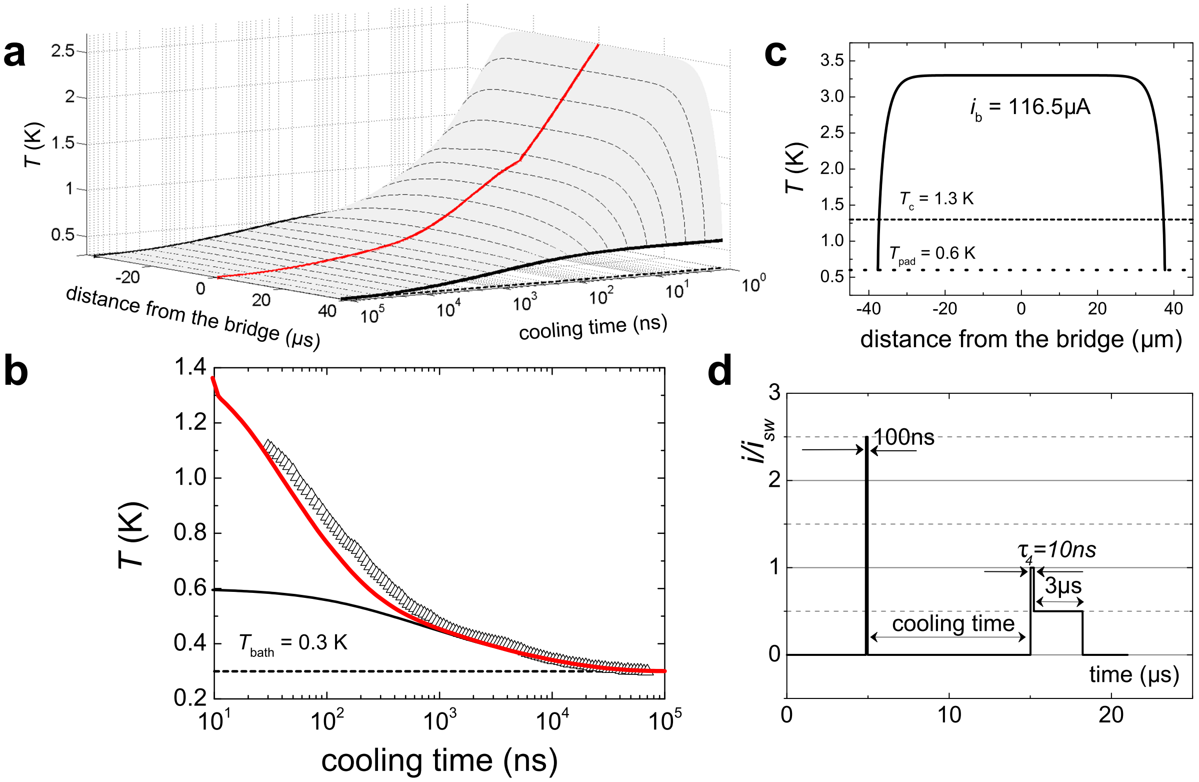


**Figure S7:** Numerical modeling of temperature relaxation in the superconducting nanowire. **(a)** Temporal evolution of the temperature profile in the wire. Temperature variations in the bridge and in the pads are distinguished with separate curves (red and black solid lines respectively). **(b)** Modeled bridge (red curve) and pad (black curve) temperatures (the same as distinguished curves from panel (a)) compared with experimental relaxation (black triangles). Cooling time $t = 0$ corresponds to the end of the heating pulse bringing the wire to a steady state with $T$=3.3 K in the center of the wire (at the nanobridge location). **(c)** Temperature profile in the wire at cooling time $t = 0$. **(d)** The layout of the pump&probe pulse used in the experiment.

## Supplementary Note 8. Numerical parameters for solving the heat flow equation in the superconducting wires: electron-phonon coupling, electron thermal conductivity and heat capacity.

### 8.1 ELECTRON-PHONON COUPLING $\dot{q}_{ep}(T_e)$

The heat flow from electrons to phonons is calculated numerically based on the integral from V. Maisi et al. PRL 111, 147001 (2013). In Figure S8a numerical calculation is plotted together with analytical solution for low temperature limit:
$\dot{q}_{ep} = \sum(T_e^5 - T_{ph}^5) \cdot e^{-\Delta/k_B T_S}$, $T_e << T_c$.

### 8.2 ELECTRON THERMAL CONDUCTIVITY FOR ALUMINUM

Thermal conductivity calculated numerically based on the integral from H.Courtois et al. Phys. Rev. Lett. 101, 067002(2008) - Figure S8b.

### 8.3 HEAT CAPACITY OF ALUMINUM

Experimental data from N.Phillips Phys. Rev. 114, 676 (1959) - Figure S8c. Note: $c(T_e > T_c) = \gamma T_e$, $\gamma = 135\,\mathrm{JK^{-2}m^{-3}}$ (instead of $90.9\,\mathrm{JK^{-2}m^{-3}}$ expected for the free electron model).

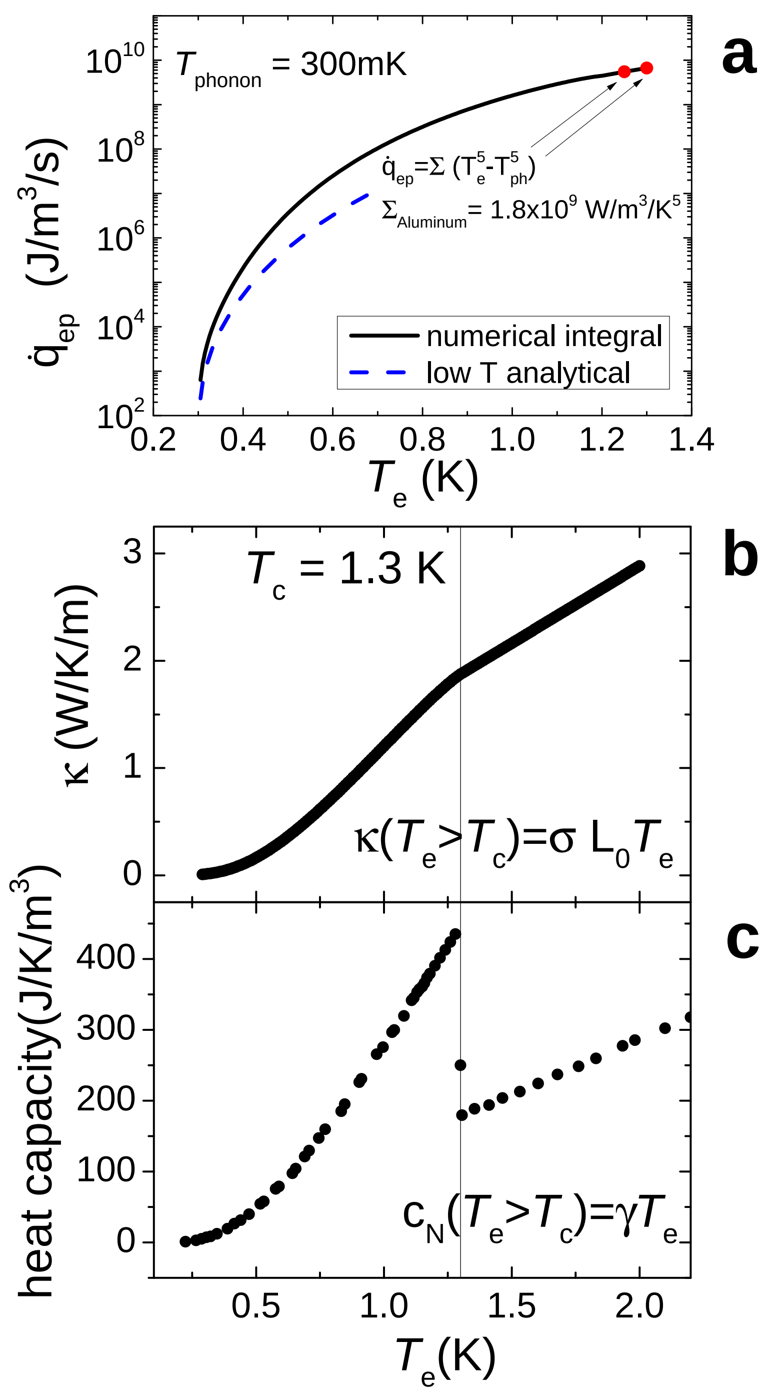


**Figure S8:** Numerical parameters used to solve heat flow equation. **(a)** Electron-phonon coupling, **(b)** Thermal conductivity, **(c)** Heat capacity.
